# Supplementary material for: Combined subleading high-energy logarithms and NLO accuracy for W production in association with multiple jets
Source: arXiv:2012.10310 source file (2021-04-08)
Supplement: Supplementary file 1 [file ExtremalQQbar.tex]

% \subsection{Derivation of the Extremal $Q \bar{Q}$ Current}
% % \subsection{Derivation}
% \label{appendix:qqbar}

\begin{figure}[t]
\centering
\includegraphics[width=0.3\textwidth]{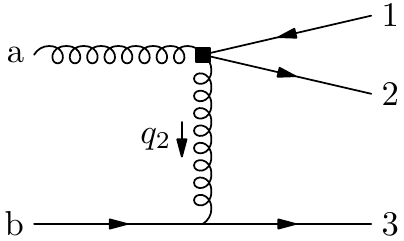}
\caption{Schematic structure of the $gq \to \bar{Q}Qq$ amplitude in the limit
  $y_1 \sim y_2 \ll y_3$ which reduces to an effective $g \to \bar{Q} Q  g^*$
  vertex and a standard \HEJ current.}
\label{fig:qgimp}
\end{figure}
